# Supplementary material for: Arbitrary control over multimode wave propagation for machine learning
Source: arXiv:2402.17750 source file (2026-06-11)

N=100  
Simulations

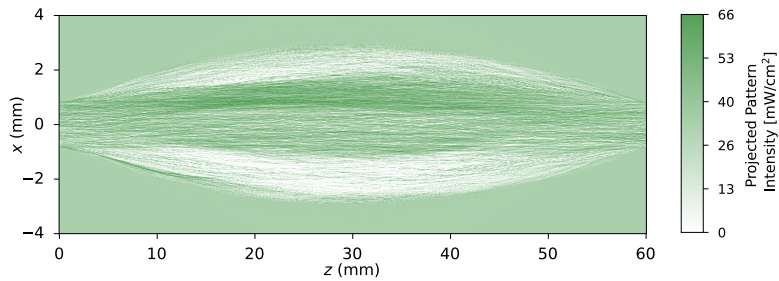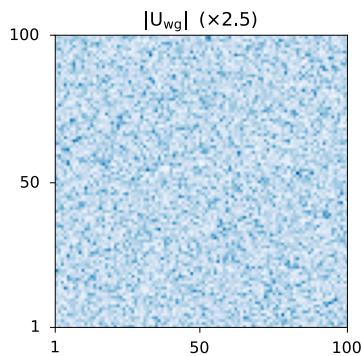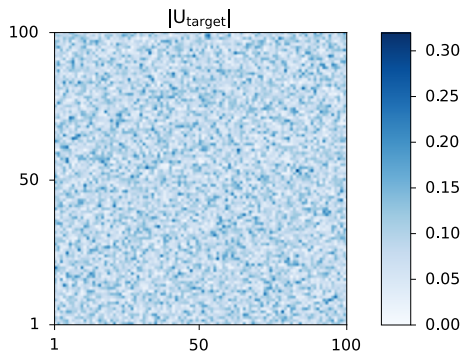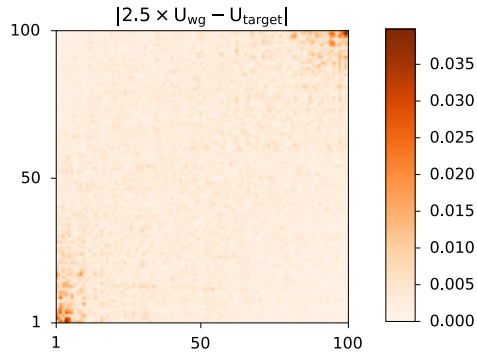

N=150  
Simulations

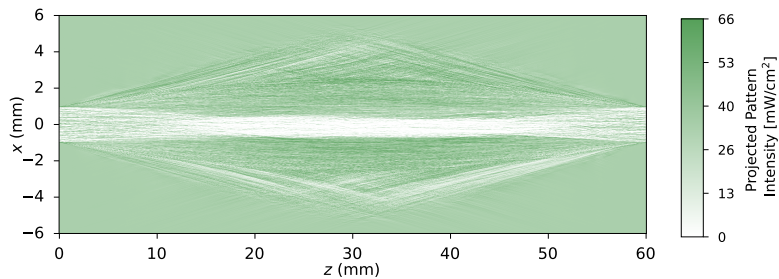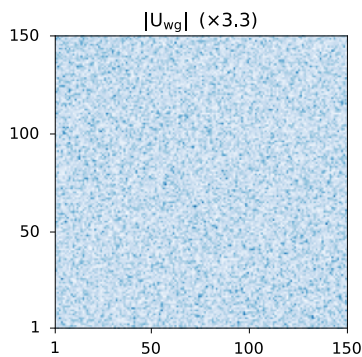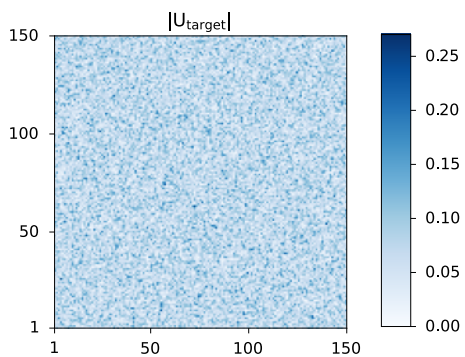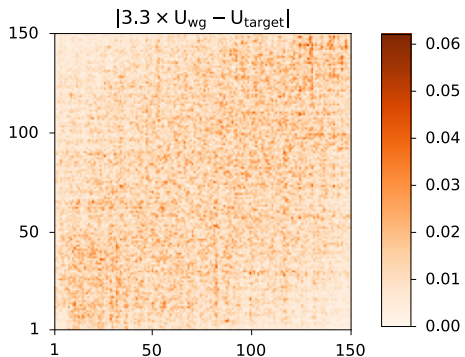

N=100  
Simulations

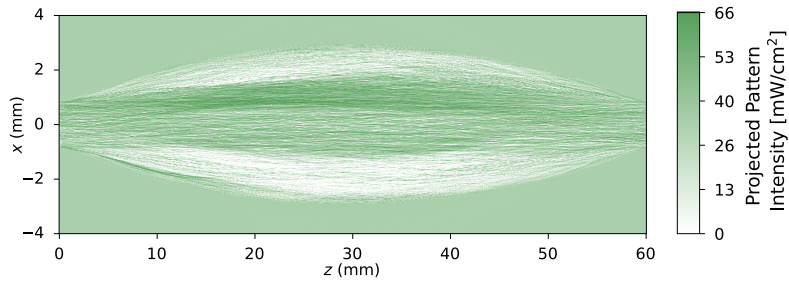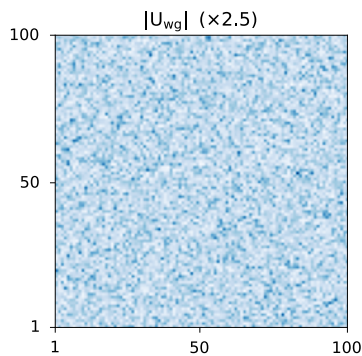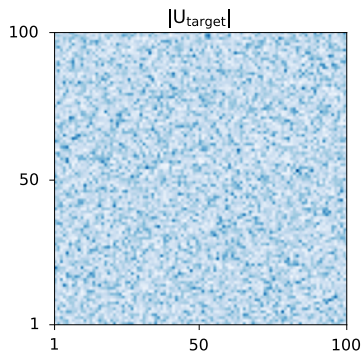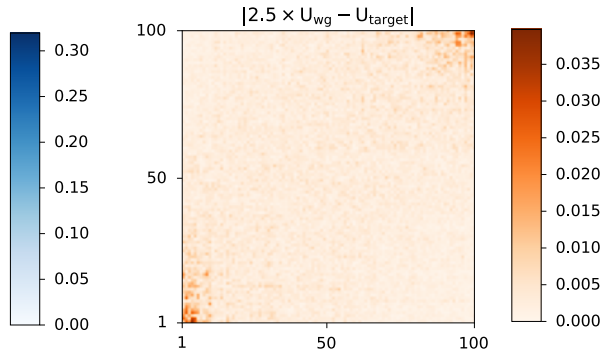

N=150  
Simulations

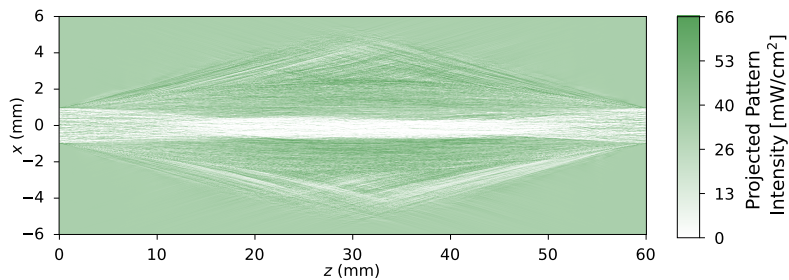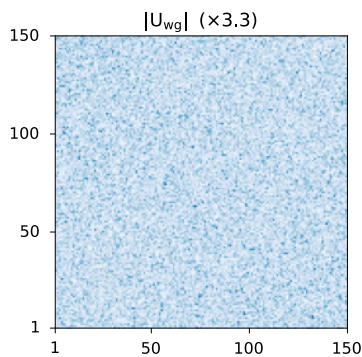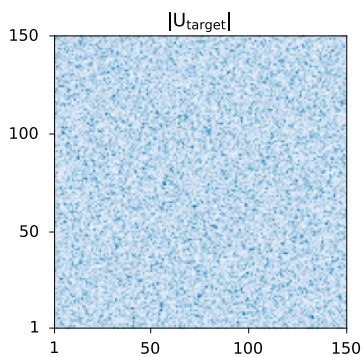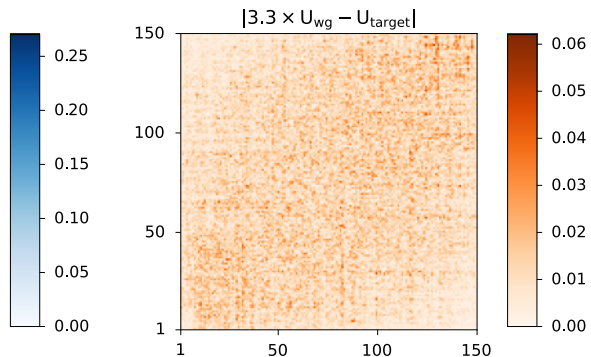

Supplement: Supplementary file 2 [file unitary_figure.pdf]
